# Supplementary material for: Factorized Fourier Neural Operators
Source: arXiv:2111.13802 source file (2023-03-02)
Supplement: Supplementary file 1 [file appendix-ns.tex]

\section{Navier-Stokes Equations}
\label{apdx:navier-stokes}

This section is written for machine learning practioners without a background
in fluid dynamics. The focus is on the implementation of the numerical methods
used as baselines in our experiments. All equations are presented in 2D.

\subsection{Useful Identities}
We can turn the differential operator in the physical space into multiplication
in the wavenumber space:
\begin{align}
  \mathcal{F}\{ \nabla \mathbf{u} \}
  =
  \mathcal{F}\bigg\{
\begin{pmatrix}
  \partial \mathbf{u} / \partial x \\
  \partial \mathbf{u} / \partial y
\end{pmatrix}
\bigg\}
=
\begin{pmatrix}
  2\pi i \kappa_x \, \mathcal{F}\{ \mathbf{u}\} \\
  2\pi i \kappa_y \, \mathcal{F}\{ \mathbf{u}\}
\end{pmatrix} \label{eqn:grad-fourier}
\end{align}
where $\kappa_x$ and $\kappa_y$ are the wavenumbers in the $x$ and $y$
dimensions, and $\mathcal{F}$ represents the Fourier transform.

Taking the Laplacian in the physical space is equivalent to multiplying its
Fourier transform by a circularly symmetric quadratic:
\begin{align}
  \mathcal{F}\{ \nabla^2 \mathbf{u} \}
= -(2\pi)^2(\kappa_x^2 + \kappa_y^2) \, \mathcal{F}\{ \mathbf{u}\}
\end{align}
Another useful identity:
\begin{align}
  \nabla \cdot (\mathbf{u} \otimes \mathbf{u}) =
    (\nabla \cdot \mathbf{u}) \mathbf{u}
    + (\mathbf{u} \cdot \nabla) \mathbf{u} \label{eqn:tensor}
\end{align}
where $\otimes$ is the tensor (or outer) product, $\mathbf{u} \otimes
\mathbf{v} = \mathbf{u} \mathbf{v}^T$.

\subsection{Stream function, velocity, and vorticity}

For a 2D flow, the stream function ${\boldsymbol\psi}$ can be defined as the
vector whose curl gives us the velocity field $\mathbf{u}$:
\begin{align}
  \mathbf{u} = \nabla \times {\boldsymbol\psi}
\end{align}
where ${\boldsymbol\psi} = (0, 0, \psi)$ and $\mathbf{u} = (u, v, 0)$. In Cartesian
coordinates, we can write this as
\begin{align}
  u = \dfrac{\partial \psi}{\partial y} \qquad\qquad v = -\dfrac{\partial \psi}{\partial x}
  \label{eqn:stream-velocity}
\end{align}
Similarly, we can define the vorticity as the curl of the velocity:
\begin{align}
  {\boldsymbol\omega} = \nabla \times \mathbf{u}
\end{align}
where ${\boldsymbol\omega} = (0, 0, \omega)$. In Cartesian coordinates, we can write this as
\begin{align}
  \omega = \dfrac{\partial v}{\partial x} - \dfrac{\partial u}{\partial y}
  \label{eqn:vorticity-velocity}
\end{align}
The Poisson equation provides a relationship between the stream function
and the vorticity:
\begin{align}
  \nabla^2 \psi = - \omega \label{eqn:poisson}
\end{align}
\cref{eqn:stream-velocity,eqn:vorticity-velocity,eqn:poisson} provide a way for
us to convert between the vorticity field and the velocity field.

\subsection{Incompressible 2D Navier-Stokes Equations}

The incompressible Navier-Stokes equations can be expressed in either
convective form,
\begin{align}
  \dfrac{\partial \mathbf{u}}{\partial t} + \mathbf{u} \cdot \nabla \mathbf{u}
    &= -\dfrac{1}{\rho} \nabla p + \nu \nabla^2 \mathbf{u} + \mathbf{f} \\
    \nabla \cdot \mathbf{u} &= 0
\end{align}
or conservation form,
\begin{align}
  \dfrac{\partial \mathbf{u}}{\partial t} + \nabla \cdot (\mathbf{u} \otimes \mathbf{u})
    &= -\dfrac{1}{\rho} \nabla p + \nu \nabla^2 \mathbf{u} + \mathbf{f} \\
    \nabla \cdot \mathbf{u} &= 0
\end{align}
The equivalence of the two forms comes from \cref{eqn:tensor} and the
conservation of mass equation, $\nabla \cdot \mathbf{u} = 0$.

By taking the curl of the Naiver-Stokes equations, we can also arrive
at the vorticity equation,
\begin{align}
  \dfrac{\partial \omega}{\partial t} + \mathbf{u} \cdot \nabla \omega
    &= \nu \nabla^2 \omega + \mathbf{f} \\
    \nabla \cdot \mathbf{u} &= 0
\end{align}
Note how the pressure term has vanished.

The kinematic viscosity $\nu$ is the ratio of the dynamic viscosity $\mu$ over
the density of the fluid $\rho$,
\begin{align}
  \nu = \dfrac{\mu}{\rho}
\end{align}
In Kolmogorov flow~\cite{Chandler2013Invariant}, the forcing function is set to
\begin{align}
  \mathbf{f} = \sin (4y) \mathbf{\hat{x}} - b \mathbf{u}
\end{align}
where $b=0.1$ models the drag force that prevents the accumulation of energy at
large scales~\cite{Boffetta2012Two}.

\subsection{Projection Method method}

In the projection method, we would like to estimate $\frac{\partial
\mathbf{u}}{\partial t}$. In the first step, we ignore the pressure gradient
term

\subsection{Pseudo-spectral method}

Each step of the numerical solver essential involves finding $\frac{\partial
\mathbf{\hat\omega}}{\partial t}$, i.e. figuring out how much the vorticity
changes in the wavenumber space when we increment time by a tiny step. It's often
convenient to break the Navier-Stokes equations into linear and non-linear
terms:
\begin{align}
  \dfrac{\partial \hat \omega }{\partial t}
= \mathbf{G}(\hat \omega) +
\mathcal{F} \big\{ \mathbf{F}(\omega) \big\}
\end{align}
In particular, the linear terms are the internal stress forces and the drag.
These are computed implicitly in the wavenumber space:
\begin{align}
  \mathbf{G}(\hat\omega)= \nu \nabla^2 \hat \omega - b \hat \omega
\end{align}
where b is the velocity-dependent drag preventing accumulation of energy at
large scales (linear term in the forcing function).
In contrast, the non-linear are computed explicitly in the physical space:
\begin{align}
  \mathbf{F}(\omega) = -\mathbf{u} \cdot \nabla \omega + \mathbf{f}
\end{align}
where $\mathbf{u} \cdot \nabla$ is the advection operator (movement of fluid)
and $\mathbf{f}$ is the non-linear terms of the forcing function. In practice,
we compute the gradient $\nabla \omega$ in the wavenumber space to take
advantage of the multiplication trick in \cref{eqn:grad-fourier}, and then we
transform back to the physical space to compute the divergent $\mathbf{u} \cdot
\nabla \omega$.

\subsection{Small-scale dissipation}

To model the small-scale dissipation, we use an circular exponential filter in
the wavenumber space~\cite{Arbic2003Coherent}:
\begin{align}
  \text{Filter} =
  \begin{cases}
    \exp\bigg(-\alpha \Big(\sqrt{k_x^2 + k_y^2} - k_N \Big)^4 \bigg)
      & \text{if $\sqrt{k_x^2 + k_y^2} > 0.65 k_N$}\\
    1 & \text{otherwise}
  \end{cases}
\end{align}
where $k_N$ is the Nyquist scale and $\alpha$ is set to
23.6~\cite{Abernathey2021pyqg}.

\subsection{CNAB}

Crank-Nicolson/Adams-Bashforth method. the Crank-Nicolson scheme for the linear
term and the Adams-Bashforth scheme for the nonlinear term

\subsection{Code}

\definecolor{bg}{rgb}{0.95,0.95,0.95}

\begin{minted}[mathescape,numbersep=5pt,bgcolor=bg,xleftmargin=5pt,xrightmargin=5pt,fontsize=\small,baselinestretch=1.1]{python}
def step_fn(omega_hat):
    # Return $\omega_{t+1}$ given $\omega_t$.
    h = 0

    # Five stages
    for k in range(len(beta)):
        h = F(omega_hat) + beta[k] * h
        mu = 0.5 * dt * (alpha[k + 1] - alpha[k])

        # Solve for equation: $\omega' - \mu G(\omega') = \omega + \gamma_k (dt) h + \mu G(\omega)$
        omega_hat = G_inv(omega_hat + gamma[k] * dt * h + mu * G(omega_hat), mu)

    return u
\end{minted}

We can see that...

\section{Old Stuff}

where $x, y \in (0, 1)$ are the positions on the unit torus,
$t \in (0, T]$ is the time step, $\nu$ is the viscosity, $v_t(x, y)$ is the
velocity field, $\omega \coloneqq \nabla \times v $ is the vorticity field, and
$f_t(x, y)$ is the forcing function. Given the forcing function
\begin{align}
  f(x, y) = 0.1 [
    \sin(2\pi (x + y)) +
    \cos(2\pi (x + y))
  ],
\end{align}
the Reynolds number is approximately
\begin{align}
Re \approx \frac{\sqrt{0.1}}{\nu
(2\pi)^{3/2}}
\end{align}

For \TorusV and \TorusVF, the forcing function on the torus is defined as
\begin{align}
  f(t, x, y) &= 0.1 \sum_{p=1}^2 \sum_{i=0}^1 \sum_{j=0}^1 \Big[
    \alpha_{pij} \sin\big( 2\pi p (i x + j y) + \delta t \big) +
    \beta_{pij} \cos\big( 2\pi p (i x + j y) + \delta t \big)
  \Big]
\end{align}
where the amplitudes $\alpha_{pij}$ and $\beta_{pij}$ are sampled from the uniform
distribution in \TorusV and \TorusVF. Furthermore, $\delta$ is set to 0 in
\TorusV, making the forcing function constant across time; while it is set to
0.2 in \TorusVF, giving us a time-varying force. Finally in \TorusZongyi, the
forcing function is fixed at
$
  f(x, y) = 0.1 [
    \sin(2\pi (x + y)) +
    \cos(2\pi (x + y))
  ]
$
across all samples and time steps.
